# Supplementary material for: XMixup: Efficient Transfer Learning with Auxiliary Samples by Cross-domain Mixup
Source: arXiv:2007.10252 source file (2020-07-20)
Supplement: Supplementary file 1 [file 7_appendix.tex]

\begin{appendices}
\appendix

\section{Beta Distribution}
\begin{figure}
  \centering
    \includegraphics[height=0.25\textwidth,width=0.9\textwidth]{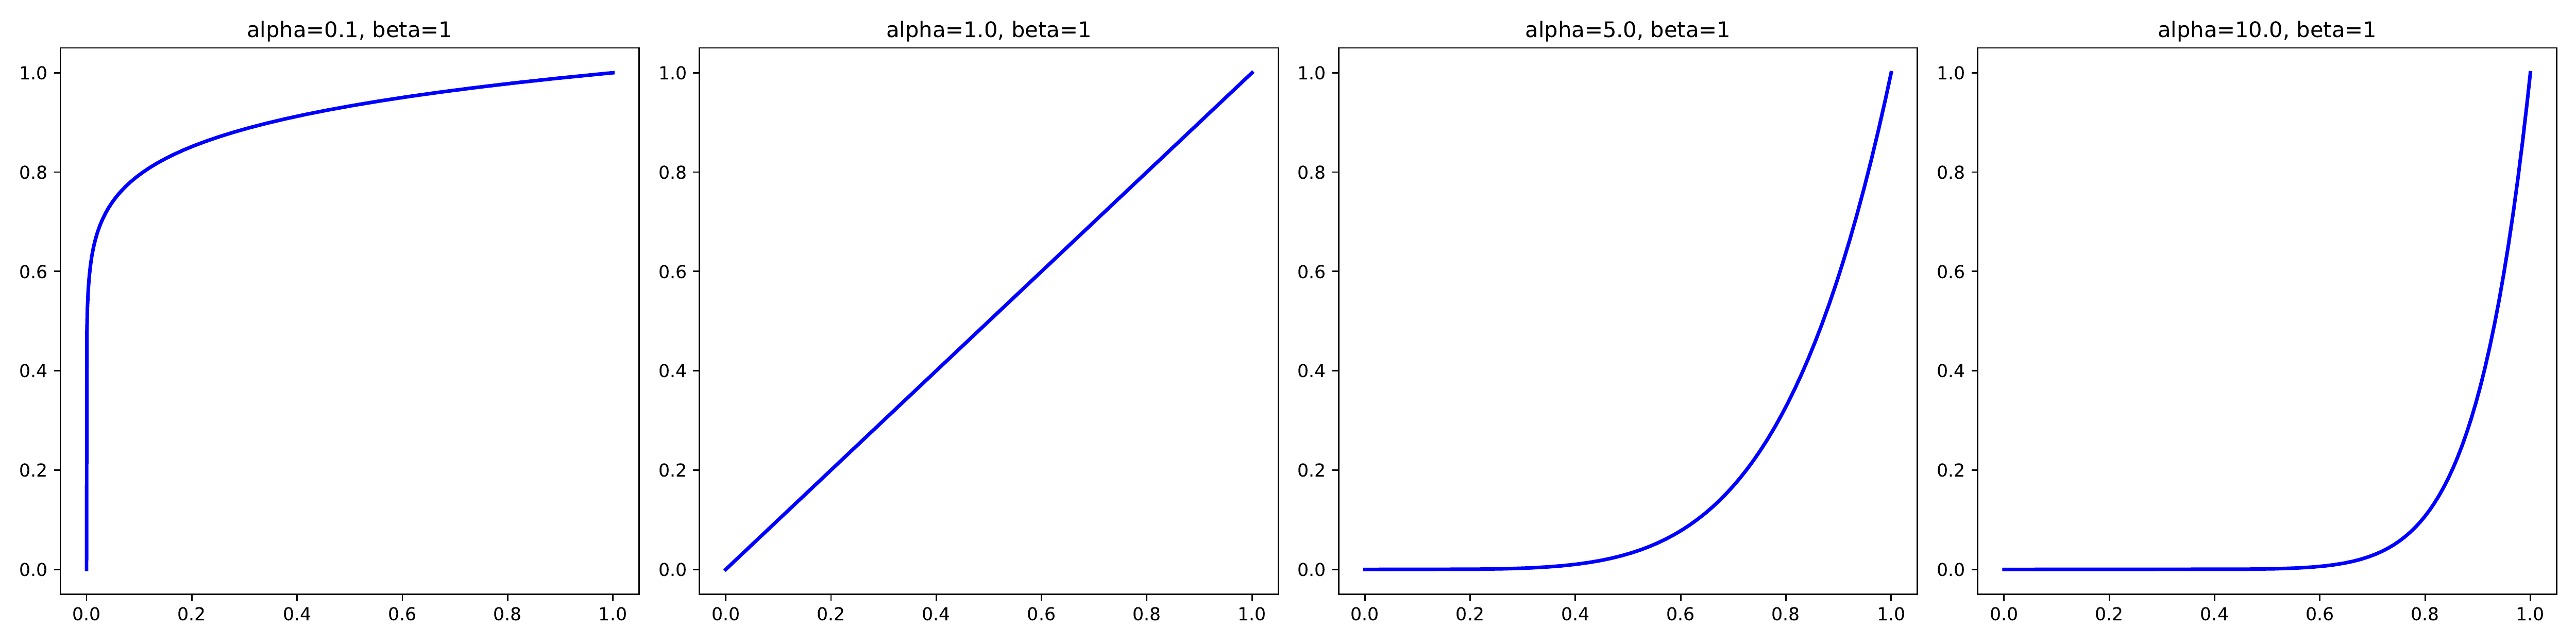}
    \caption{Examples of Beta Distribution.}
    \label{fig:svd}
\end{figure}

\end{appendices}
